# Supplementary material for: Improving Viewpoint Consistency in 3D Generation via Structure Feature and CLIP Guidance
Source: arXiv:2412.02287 source file (2025-08-14)
Supplement: Supplementary file 1 [file supp_sec.tex]

\clearpage
\setcounter{page}{1}
\maketitlesupplementary

\section{Formula Derivation }
\label{sec:formula}

Assume that the initial data distribution \( p_{\text{data}}(x) \) follows a long-tailed distribution. We aim to prove that \( q_{\text{generation}}(x) \) also follows a long-tailed distribution.

\subsection{Forward process}
We know the SDE of the forward Diffusion process was given by~\cite{song2020score}:

\begin{equation}
dx = f(x, t)dt + g(t)dW \tag{1}
\end{equation}

From this, we derive the Fokker-Planck equation~\cite{oksendal2013stochastic, risken1996fokker} which governs the time evolution of the probability density function \( p_t(x) \):

\begin{equation}
\frac{\partial p_t(x)}{\partial t} = -\nabla_x \cdot \left( f(x, t) p_t(x) \right) + \frac{1}{2} g(t)^2 \nabla_x^2 p_t(x) \tag{2}
\end{equation}

Next, we present the gradient formula linking the log-density gradient to the density gradient:

\begin{equation}
\nabla_x \log p_t(x) = \frac{\nabla_x p_t(x)}{p_t(x)}
\tag{3}
\label{equation3}
\end{equation}

Substituting this into the diffusion term gives:

\[
\frac{1}{2} g(t)^2 \nabla_x^2 p_t(x) = \frac{1}{2} g(t)^2 \nabla_x \cdot \left( p_t(x) \nabla_x \log p_t(x) \right)
\]

Finally, we combine the diffusion and drift terms by substituting the above result into the Fokker-Planck equation:

\[
\frac{\partial p_t(x)}{\partial t} = \begin{aligned}[t]
&- \nabla_x \cdot \left( f(x, t) p_t(x) \right) \\
&+ \nabla_x \cdot \left( \dfrac{1}{2} g(t)^2 p_t(x) \nabla_x \log p_t(x) \right)
\end{aligned}
\]
By merging the two divergence terms, we arrive at the final form of the Fokker-Planck equation:

\begin{equation}
\frac{\partial p_t(x)}{\partial t} = -\nabla_x \cdot \left[ \left( f(x, t) - \frac{1}{2} g(t)^2 \nabla_x \log p_t(x) \right) p_t(x) \right] \tag{4}
\label{equation4}
\end{equation}

\subsection{Reverse process}

We know the SDE of the reverse Diffusion process was given by~\cite{song2020score}:

\begin{equation}
dx = \left[f(x, t) - g(t)^2 \nabla_x \log p_t(x)\right] dt + g(t) d\Bar{w} \tag{5}
\end{equation}

Assuming the initial \( q_T(x) \sim \mathcal{N}(0, 1) \), we aim to determine how \( q_t(x) \) evolves over the time interval \( t \in [T, 0] \).

To facilitate this, we introduce a new time variable \( s = T - t \), where \( s \) increases from \( 0 \) to \( T \) as \( t \) decreases from \( T \) to \( 0 \). Consequently, the differential relationship becomes:

\[
ds = -dt
\]

Rewriting the reverse SDE in terms of the new time variable \( s \), we obtain:

\begin{equation}
dx = \left[-f(x, t) + g(t)^2 \nabla_x \log p_t(x)\right] ds + g(t) d{w} \tag{6}
\end{equation}

Here, \( d{w} \) represents a forward Wiener process in the new time \( s \).
\begin{figure*}[htbp]
    \centering
    \includegraphics[width=\linewidth]{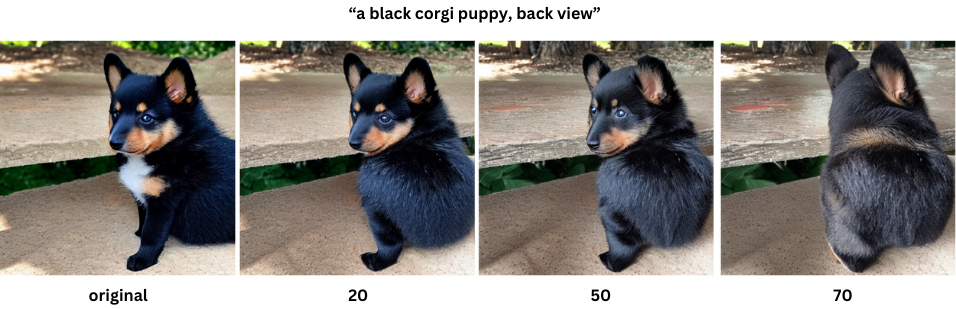}
    \caption{As the cross attention control ratio for token “back” increases, the front features gradually disappear and the back features emerge.}
    \label{fig:sup_1}
\end{figure*}
Using the Fokker-Planck equation, the evolution of \( q_s(x) \) with respect to time \( s \) is described by:

\begin{equation}
\begin{aligned}
\frac{\partial q_s(x)}{\partial s} ={} & -\nabla_x \cdot \left\{ q_s(x) \left[ -f(x, t) + g(t)^2 \nabla_x \log p_t(x) \right] \right\} \\
&\quad + \frac{1}{2} g(t)^2 \nabla_x^2 q_s(x)
\end{aligned}
\tag{7}
\end{equation}

Using Eq.~\ref{equation3}, we have:

\begin{equation}
\begin{aligned}
\frac{\partial q_s(x)}{\partial s} = 
\nabla_x \cdot \Big[ \Big( & f(x, t) 
- g(t)^2 \nabla_x \log p_t(x) \\
& + \frac{1}{2} g(t)^2 \nabla_x \log q_s(x) \Big) q_s(x) \Big]
\end{aligned}
\tag{8}
\end{equation}

The forward time step \( t \) and the reverse time step \( s \) represent the same point in time.
The key to the reverse process, inverting the forward process, lies in accurately estimating the score function \( \nabla_x \log p_{t}(x) \). In practice, this estimation is performed by training a neural network to approximate the true score function. If the neural network provides an accurate estimate:

\[
\begin{aligned}
\nabla_x \log q_s(x) \approx \nabla_x \log p_t(x)
\end{aligned}
\]

Finally, rearranging the terms leads to:

\begin{equation}
\frac{\partial q_s(x)}{\partial s} = -\nabla_x \cdot \left[ \left( \frac{1}{2} g(t)^2 \nabla_x \log p_t(x) - f(x, t) \right) q_s(x) \right] \tag{9}
\label{equation9}
\end{equation}

\subsection{Evolution of Data Distribution Over Time}
From the perspective of \textbf{probability flow density}, the Fokker-Planck equation describes how the probability density function (PDF) evolves over time under stochastic dynamics. In our derivation, we obtained the Fokker-Planck equation for the forward SDE as shown in equation (4):

\[
\frac{\partial p_t(x)}{\partial t} = -\nabla_x \cdot \left[ \left( f(x, t) - \frac{1}{2} g(t)^2 \nabla_x \log p_t(x) \right) p_t(x) \right]
\]

This equation characterizes the time evolution of the probability density \( p_t(x) \) influenced by the drift term \( f(x, t) \) and the diffusion term involving the gradient of the log-density \( \nabla_x \log p_t(x) \).

In the reverse process, we introduce a new time variable \( s = T - t \) to effectively reverse the time direction. The Fokker-Planck equation for the reverse SDE, derived in equation (9), is given by:

\[
\frac{\partial q_s(x)}{\partial s} = -\nabla_x \cdot \left[ \left( \frac{1}{2} g(t)^2 \nabla_x \log p_t(x) - f(x, t) \right) q_s(x) \right]
\]

Here, the drift and diffusion terms have signs opposite to those in the forward equation, and the time derivative is with respect to \( s \), reflecting the reversal of time. 

From the probability flow density viewpoint, this sign reversal implies that the reverse Fokker-Planck equation effectively inverts the probability flow dictated by the forward equation. The probability density \( q_s(x) \) in the reverse process evolves in a manner that retraces the evolution of \( p_t(x) \) in the forward process but in reverse time. This ensures that the reverse SDE undoes the effect of the forward SDE on the probability density, allowing the generative distribution \( q_{\text{generation}}(x) \) to approximate the original data distribution \( p_{\text{data}}(x) \).

Therefore, based on our derivations leading to equations~\ref{equation4} and~\ref{equation9}, we can conclude that the Fokker-Planck equation for the reverse SDE is indeed the reverse process of the forward SDE's Fokker-Planck equation. This explains how the reverse diffusion process successfully reconstructs samples from the data distribution by inverting the probability flow of the forward process. This also reveals that the long-tail distribution of the training data of the diffusion model affects the distribution of the generated data.

\section{Experimental details}
\subsection{Implementation Details}
\noindent \textbf{Cross-Attention Controlling.} 
Building upon image editing techniques based on diffusion models~\cite{hertz2022prompt}, we find that controlling the cross-attention map can control generation outcomes. In our 2D image generation experiments, modifying viewpoint-specific keywords like \textit{``back''} allows us to transform front-facing images into accurate back-view perspectives without changing the image's structure or subject. Therefore, we propose that controlling cross-attention can reduce viewpoint bias and improve 3D optimization balance. Figure~\ref{fig:sup_1} illustrates the effects of adjusting weights to gradually remove positive features.

We employ the random uniform viewpoint sampling strategy from DreamFusion, with rotation angle ranges defined for front, side, and back views as $[-60^\circ, 60^\circ)$, $[-120^\circ, -60^\circ) \cup [60^\circ, 120^\circ)$, and $[-180^\circ, -120^\circ) \cup [120^\circ, 180^\circ)$, respectively. To emphasize side and back views, we apply weighting factors of $5 \times \text{prompt length}$ and $10 \times \text{prompt length}$, respectively. We modify the \texttt{AttnProcessor2} method in Diffusers to reweight the cross-attention map accordingly.

\noindent \textbf{CLIP Pruning.} 
We attribute the Janus Problem to the long-tail distribution in training data, allowing us to apply methods designed for such distributions. We identify two strategies to address long-tail issues: modifying classifiers and rebalancing sampling. Although classifier guidance~\cite{dhariwal2021diffusion} inspired us, initial experiments using CLIP guidance to generate tail classes~\cite{sehwag2022generating} were unsuccessful due to the generic Open-CLIP~\cite{ilharco_gabriel_2021_5143773,radford2021learning} not being trained on noisy images.

Therefore, we adopt a rebalanced sampling strategy. We treat all pseudo-ground truth outputs from the diffusion model as a potential optimization database, which is imbalanced in front, side, and back views. Unlike DreamControl~\cite{huang2024dreamcontrol}, which rebalances sampling ratios based on computed confidence intervals, we rebalance optimization by pruning incorrect viewpoint images without explicitly calculating confidence intervals.

In our experiments, we used the viewpoint classifications of \textit{``front view,''} \textit{``side view,''} and \textit{``back view,''} converting them into textual embeddings using CLIP. For each iteration, we transformed the pseudo-ground truth \( \bar{x}_0 \) from latent space to pixel space via the VAE. We then embedded the resulting image using CLIP to compute its similarity with the viewpoint embeddings.

\noindent \textbf{Coarse to Fine.} This prompt-based optimization strategy was proposed due to the diffusion model's limited ability to comprehend long prompts.  To address this, we split complex prompts into two components: a simple object description and a descriptive short phrase. During the initial stages, we focus on optimizing the geometric features of the object itself. This process can be regarded as a simplified version of 3D editing techniques.

\begin{figure}[!htbp]
    \centering
    \includegraphics[width=1\linewidth]{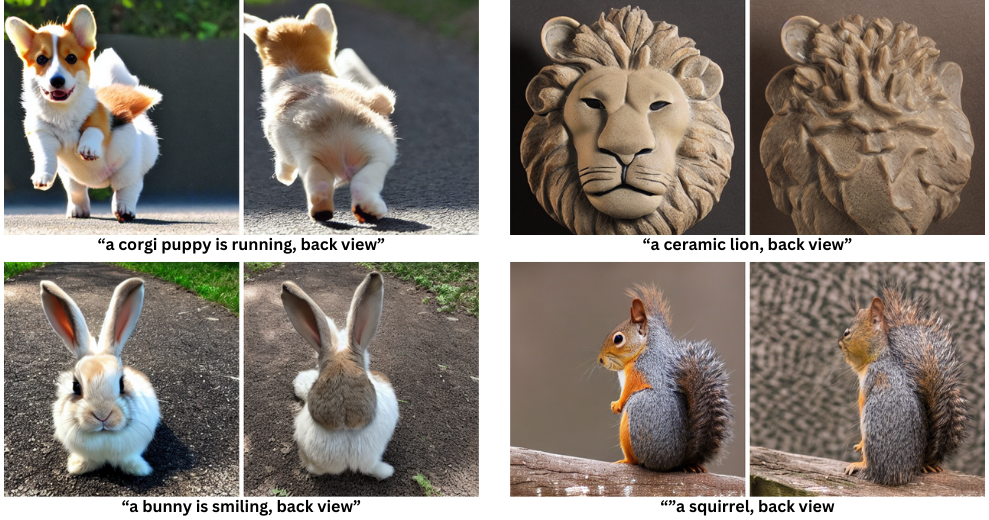}
    \vspace{-0.8em}
    \caption{By increasing the weight of the token "back," previously misgenerated images were able to produce accurate back-view features. The left side shows the original generation by SD1.4 for the given prompt, while the right side displays the results after amplifying the weight of ``back."}
    \vspace{-1.0em}
    \label{fig:sup_2}
\end{figure}

\begin{figure*}[!htbp]
    \centering
    \includegraphics[width=0.8\linewidth]{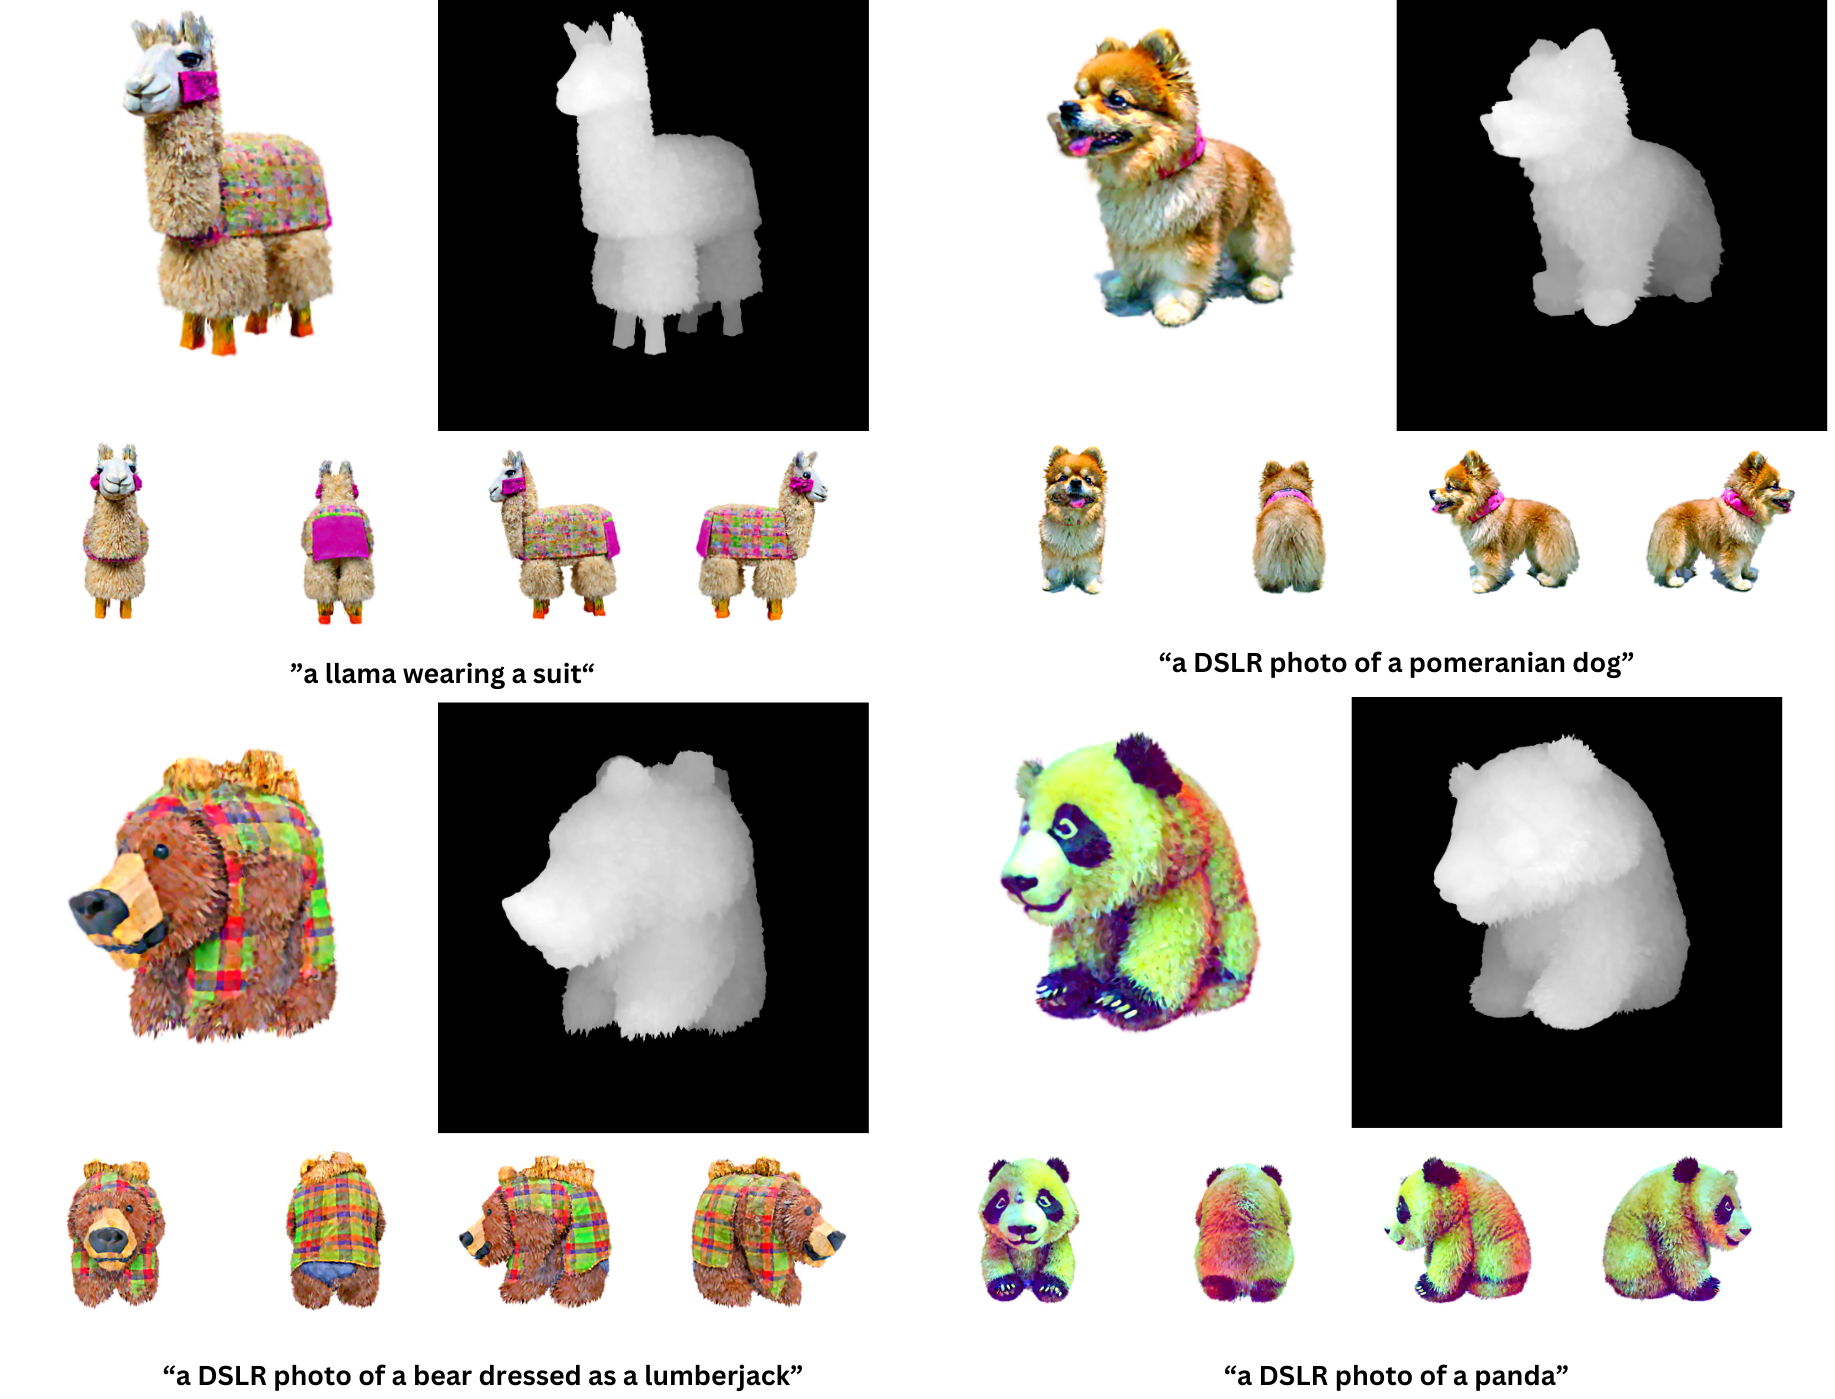}
    \caption{Additional SFCG generation.}
    \vspace{-1.0em}
    \label{fig:sup_3}
\end{figure*}
\subsection{Evaluation Metrics}
\noindent \textbf{Janus Rate.} 
To evaluate geometric consistency, we calculated the occurrence rate of the Janus Problem (JR), defined as the presence of multiple distinct front-view features, such as faces, ears, or noses.
\noindent \textbf{View Dependent CLIP-Score.} 
The CLIP-Score (CS), based on CLIP similarity, measures generation quality by evaluating the similarity between the rendered images of the generated object and the input prompt. However, this metric is not suitable for directly assessing geometric inconsistencies, as front-facing features can significantly boost image-text similarity, even when these features erroneously appear on the object's back.

To address this issue, we designed a view-dependent CLIP-Score. Following the same viewpoint classifications, we append \textit{``* view''} to the original prompt, where * represents \textit{``front,''} \textit{``side,''} or \textit{``back.''} We then render four images of the 3D object from viewpoints at \(0^\circ\), \(90^\circ\), \(180^\circ\), and \(270^\circ\) and calculate their similarities with the modified prompts respectively. The final score is computed as the mean of these similarity scores.

\section{Additional quantitative studies}
\begin{figure*}[!htbp]
    \centering
    \includegraphics[width=0.8\linewidth]{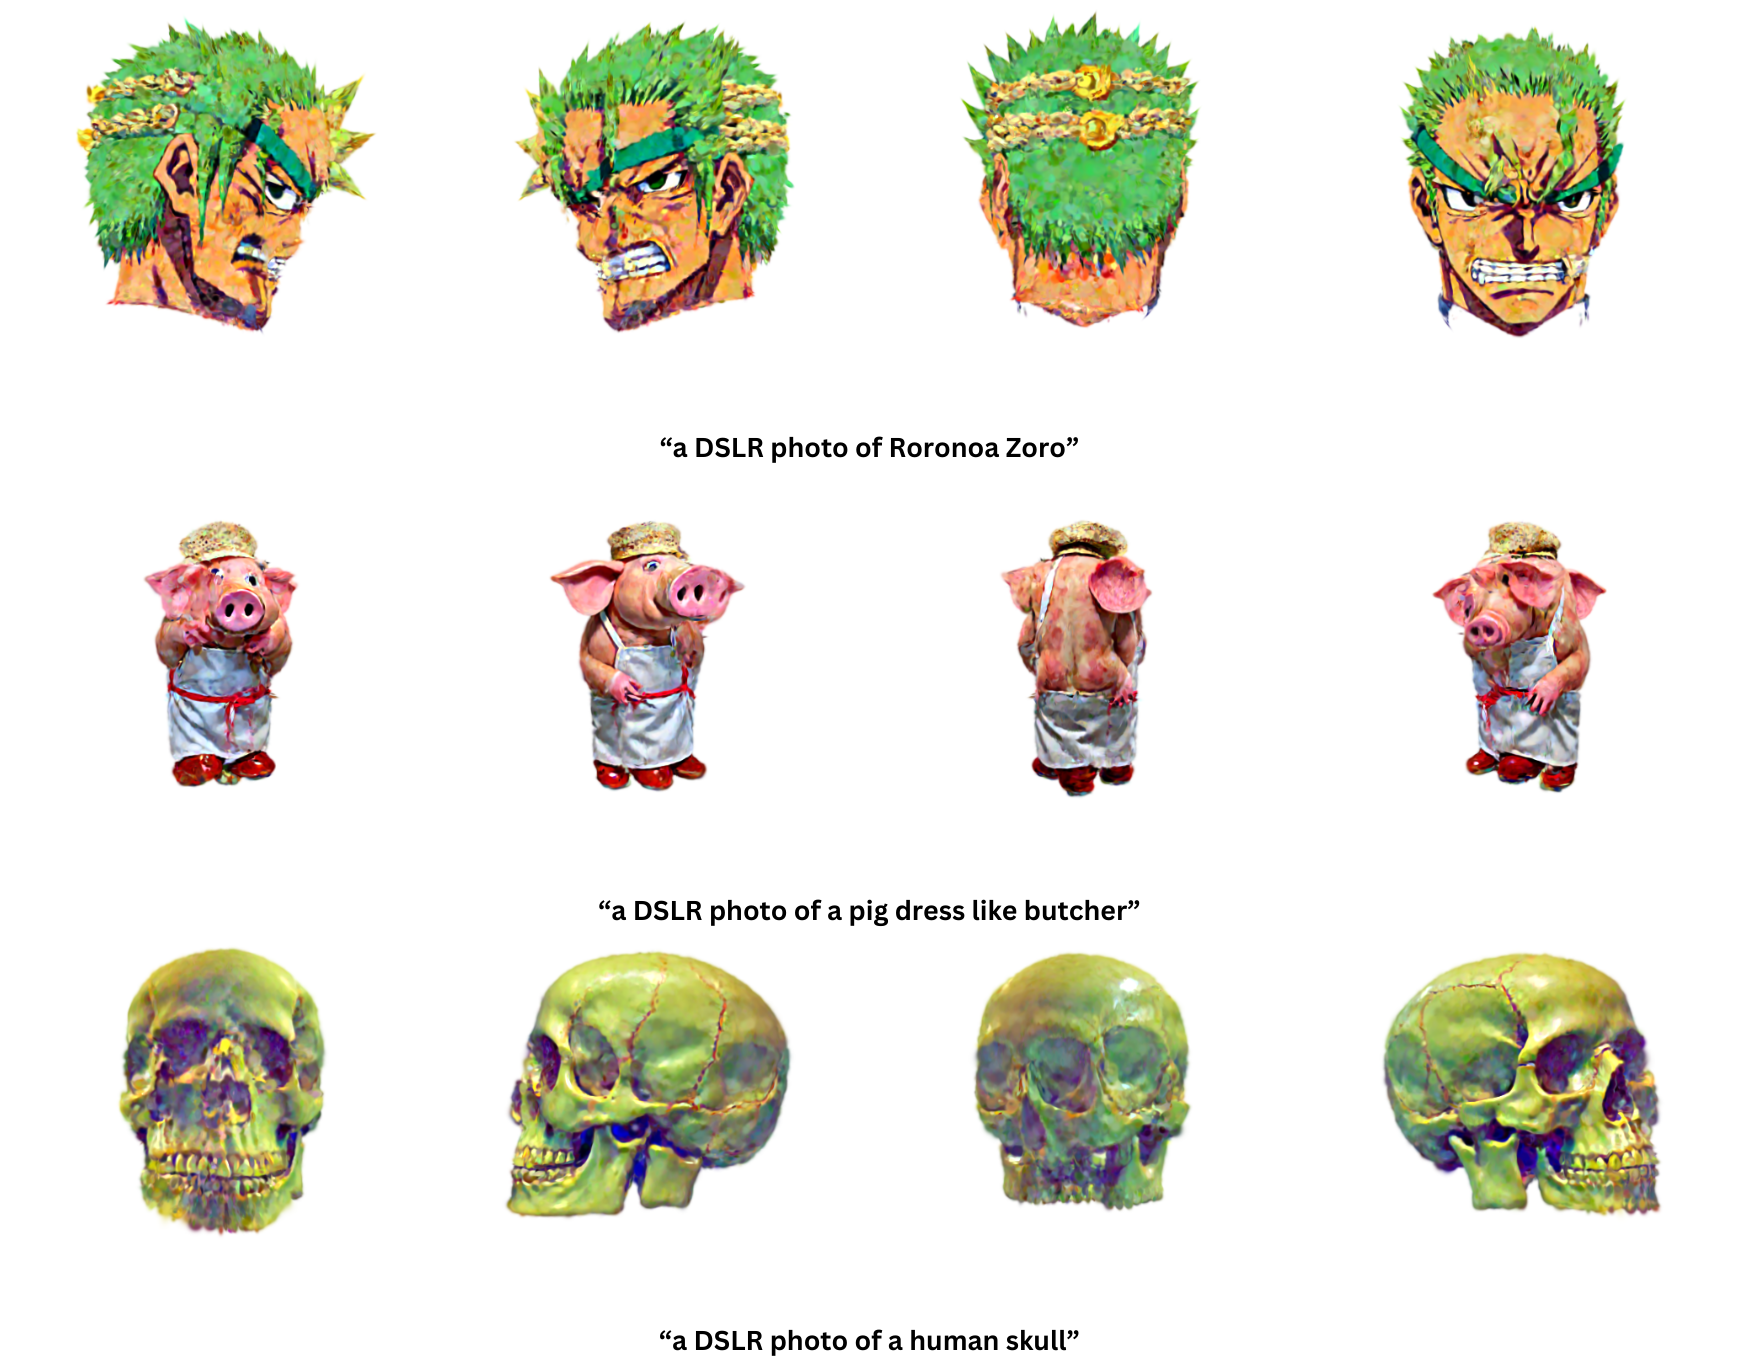}
    \caption{Failure Case}
    \vspace{-1.0em}
    \label{fig:sup_4}
\end{figure*}

In this section, we conducted a detailed evaluation of the effectiveness of each component in SFCG. First, we compared the impact of different versions of Stable Diffusion on the Janus Problem. Subsequently, we performed additional ablation studies on the individual components. 

Using DreamFusion~\cite{poole2022dreamfusion} as the baseline, we randomly generated “a DSLR photo of a corgi puppy” five times and calculated the average of the Janus Rate.

\subsection{Comparison of different SD versions}

In the random generation experiment, the baseline of SD1.4~\cite{rombach2022high} has Janus Problem for all generations. The Janus problem of SD2.1 is smaller than that of SD1.4, but still obvious.
SFCG has shown an obvious mitigation effect on the Janus Problem in both versions.

\begin{table}[!htbp]
\centering
\begin{tabular}{|c|c|c|}
\hline
   & SD1.4 & SD2.1 \\ \hline
Dreamfusion & 100\% & 60\% \\ \hline
Dreamfusion+SFCG & 40\% & 20\% \\ \hline
\end{tabular}
\caption{Qualitative comparison of the effects of SFCG on different versions of Stable Diffusion}
\label{tab:example_table}
\end{table}

\subsection{Quantitative ablation comparison}

We conducted experiments by individually adding each of the three components. All three methods demonstrated mitigation effects on the Janus Problem. The experiment was also an average of five randomly generated in DreamFusion.

\begin{table}[!htbp]
\centering
\begin{tabular}{|c|c|c|}
\hline
   & JR \\ \hline
Dreamfusion & 100\%  \\ \hline
+structure feature & 40\%  \\ \hline
+CLIP & 80\%  \\ \hline
% +Coarse to Fine & 60\%  \\ \hline
\end{tabular}
\caption{Qualitative comparison of the effect of different components of SFCG.}
\label{tab:example_table}
\end{table}

\section{More Visualization Results}
Figure~\ref{fig:sup_3} presents additional visual results. The attached video shows the 360-degree comparison with LucidDreamer Baseline.

\section{Failure Case}
Figure~\ref{fig:sup_4} shows some of our failure cases. This can be summarized as follows: the Janus problem on the back is  gone, but there are additional frontal features such as eyes or ears at the transition between the front and the side. We think that the reasons may lie in two aspects. First, side-view images in the training data of diffusion models often contain partial frontal features. Second, when adjusting the weights of cross-attention, this region is typically deprioritized.
